# Supplementary material for: Solvation Lies Within: Simulating Condensed-Phase Properties from Local Electronic Structures
Source: arXiv:2601.08649 ancillary file (2026-01-13)
Supplement: Supplementary file 1 [file si.pdf]

# Supporting Information: Solvation Lies Within: Simulating Condensed-Phase Properties from Local Electronic Structures

Kasper F. Schaltz,[†] Jonas Greiner,[†] Filippo Lipparini,[‡] and Janus J. Eriksen[*,†]

†*DTU Chemistry, Technical University of Denmark*

*Kemitorvet Bldg. 206, 2800 Kgs. Lyngby, Denmark*

‡*Dipartimento di Chimica e Chimica Industriale, Università di Pisa*

*Via G. Moruzzi 13, Pisa, 56124, Italy*

E-mail: janus@dtu.dk

# 1 Atomic Decompositions

We here briefly revisit how a total KS-DFT molecular energy (e.g., for a bulk) may be partitioned amongst the atomic nuclei of a chemical system before, in turn, being summed up into individual monomer energies. Such a decomposition may operate in terms of the spatial locality of either molecular or atomic orbitals (MOs and AOs, respectively).

## 1.1 MO-Based Decomposition

As outlined in Ref. S1, the KS-DFT energy functional for a system of $\mathcal{M}$ atoms reads

$$E = \sum_{K}^{\mathcal{M}} E_{\text{elec},K}(\boldsymbol{D}, \boldsymbol{\delta}_K) + E_{xc,K}(\boldsymbol{\rho}, \boldsymbol{\varrho}_K) + E_{\text{nuc},K} \ . \tag{S1}$$

For a closed-shell system, the nuclear and electronic contributions of Eq. S1 are defined as

$$E_{\text{nuc},K} = \frac{Z_K}{2} \sum_{L \neq K}^{\mathcal{M}} \frac{Z_L}{|\boldsymbol{r}_K - \boldsymbol{r}_L|} \tag{S2a}$$

$$E_{\text{elec},K} = \text{Tr}[\boldsymbol{T}_{\text{kin}} \boldsymbol{\delta}_K] + \frac{1}{2}(\text{Tr}[\boldsymbol{V}_K \boldsymbol{D}] + \text{Tr}[\boldsymbol{V}_{\text{nuc}} \boldsymbol{\delta}_K]) + \frac{1}{2} \sum_{\sigma} \text{Tr}[\boldsymbol{G}_\sigma(\boldsymbol{D}) \boldsymbol{\delta}_{K,\sigma}] \tag{S2b}$$

$$E_{xc,K} = \text{Tr}[\epsilon_{xc}(\boldsymbol{\rho}) \boldsymbol{\varrho}_K] \ . \tag{S2c}$$

In Eq. S2a, $Z_K$ and $\boldsymbol{r}_K$ denote the nuclear charge and position of atom $K$, while the kinetic energy and nuclear attraction operators in Eq. S2b are denoted by $\boldsymbol{T}_{\text{kin}}$ and $\boldsymbol{V}_{\text{nuc}}$, respectively, alongside the attractive potential associated with atom $K$, $\boldsymbol{V}_K$, and an effective Fock potential, $\boldsymbol{G}_\sigma$ ($\sigma = \alpha, \beta$ is an electronic spin index). In Eq. S2b, $\boldsymbol{D}$ denotes the full, spin-summed 1-electron reduced density matrix (1-RDM), while the objects that principally define this decomposition—the atom-specific 1-RDMs, $\{\boldsymbol{\delta}\}$—are constructed as follows:

$$\boldsymbol{\delta}_K = \sum_{\sigma} \boldsymbol{\delta}_{K,\sigma} = \sum_{\sigma} \sum_{i}^{\mathcal{N}_\sigma} \boldsymbol{d}_{i,\sigma} \boldsymbol{p}_{i,\sigma}^K \ . \tag{S3}$$

In turn, these are formulated via a set of 1-RDMs, $\boldsymbol{d}_{i,\sigma} = \boldsymbol{C}_{i,\sigma}\boldsymbol{C}^T_{i,\sigma}$, unique to the individual occupied spin-$\sigma$ MOs of the system, $\boldsymbol{C}_{i,\sigma}$, and a set of weights of all $\mathcal{N}_\sigma$ MOs of $\alpha$-/$\beta$-spin on a given atom $K$, $\{\boldsymbol{p}^K\}$. Our earlier investigations in Refs. S1–S7 have convincingly indicated how the atomic weights used to assign $\{\boldsymbol{d}\}$ should ideally not be drawn from regular Mulliken population analyses,[S8] but rather recast into a basis of reduced dimension. The *xc* energy in Eq. S2c is expressed in terms of the computed energy density, $\epsilon_{xc}$, as derived from the total electronic density, $\boldsymbol{\rho}$, and possibly its derivatives, which are all quantities that may be trivially defined in an atom-specific manner, $\{\boldsymbol{\varrho}\}$, by proceeding through $\{\boldsymbol{\delta}\}$.

When using $\omega$B97M-V to calculate Eq. S1,[S9] the *xc* energy in Eq. S2c comprises also a non-local contribution from the VV10 functional,[S10] in which case we add a van der Waals (vdW) contribution associated with atom $K$, given as half the total vdW energy between the QM and MM regions from the buffered 7-14 Lennard-Jones potential of AMOEBA,[S11]

$$\delta E_{\mathrm{vdW},K} = \frac{1}{2}\sum_{J}^{\mathcal{M}'} \mathcal{E}_{KJ}\Big(\frac{1+\lambda}{\mathcal{R}_{KJ}+\lambda}\Big)^7\Big(\frac{1+\gamma}{\mathcal{R}^7_{KJ}+\gamma}-2\Big) \ . \tag{S4}$$

In Eq. S4, $J$ is an atom in the MM region (of $\mathcal{M}'$ sites), while $\mathcal{R}_{KJ} = r_{KJ}/R^0_{KJ}$, $\lambda = 0.07$, and $\gamma = 0.12$. Here $r_{KJ}$ is the distance between atoms $K$ and $J$, while $R^0_{KJ}$ is the minimum energy distance. $\mathcal{E}_{KJ}$ denotes the depth of the energy potential well of a given pair of atoms.

Finally, using the notation of Eq. 1 of the main work (cf. Fig. 2), we can write the decomposed energy of monomer $\mathcal{K}$ as follows:

$$\mathcal{E}^{(n)}_{\mathcal{K}} = \mathcal{E}^{(n)}_{\mathrm{S1},\mathcal{K}} + \delta E_{\mathrm{vdW},\mathcal{K}} \ , \tag{S5}$$

while our BSSE correction, in turn, reads

$$\delta E_{\mathrm{BSSE},\mathcal{K}} = E^{(0)}_{\mathcal{K}} - E^{(0,\mathrm{G})}_{\mathcal{K}} \ . \tag{S6}$$

In Eq. S5, the contributions from Eqs. S1 and S4 have been implicitly summed for all $K \in \mathcal{K}$, and $(n)$ indicates a decomposition on $\mathcal{K}$ in the presence of $n$ surrounding monomers.

### 1.2 AO-Based Decomposition

In an AO-based decomposition, the total energy is instead partitioned amongst the constituent atoms on the basis of the full 1-RDM. In the so-called energy density analysis (EDA) by Nakai,[S12,S13] $\boldsymbol{D}$ is partitioned on account of which atoms the individual AOs are localized on (that is, irrespective of further population measures) by limiting trace operations in Eqs. S2 to only those AOs that are spatially assigned to atom $K$. In Fig. 1 of the main text, we compare the use of Eqs. S1 and S2 to the original EDA scheme. However, it should be noted how this scheme has since been extended by employing either natural atomic orbitals or real-space grids,[S14,S15] both of which ameliorate the excessive basis-set dependence of the theory somewhat (albeit at the potential expense of numerical exactness, cf. Ref. S15).

## 2 Additional Results

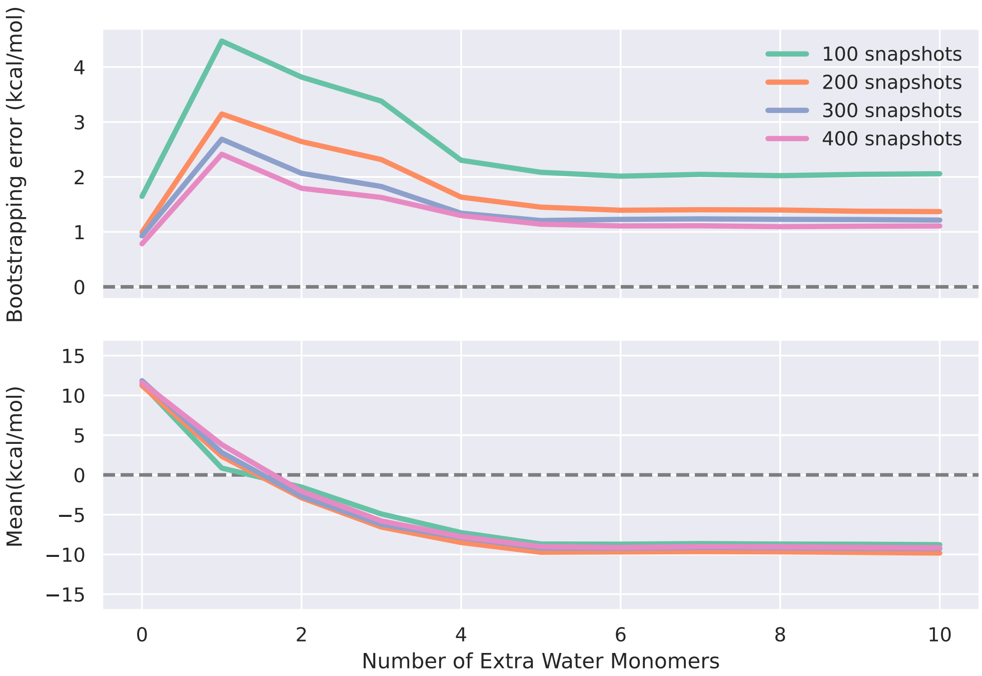


Figure S1: Bootstrapping errors for water (ωB97M-V/aug-pcseg-1).

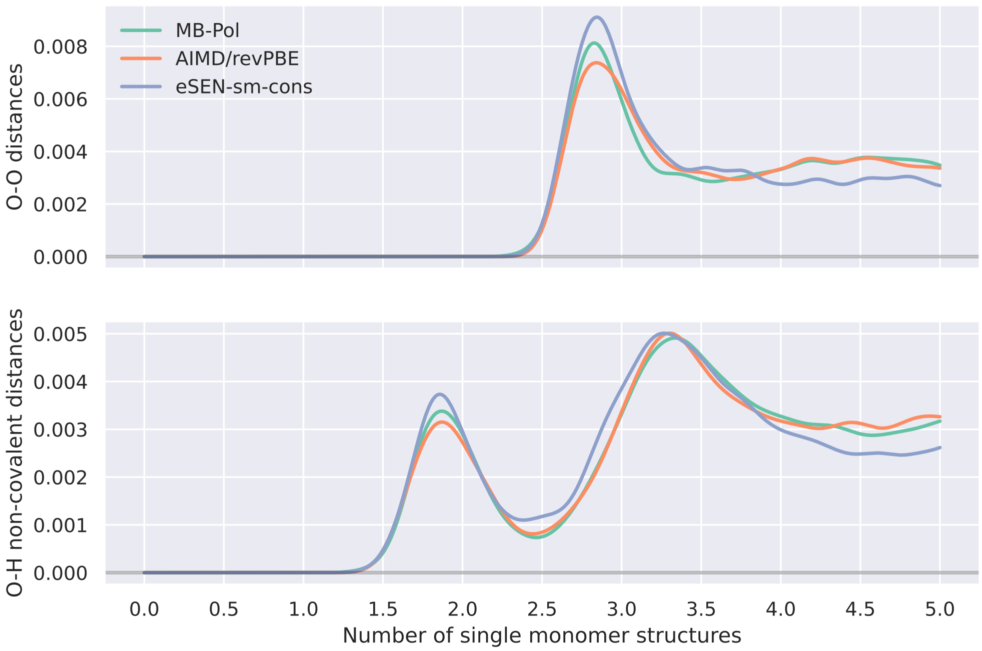


Figure S2: Radial distribution functions of different water samplings.

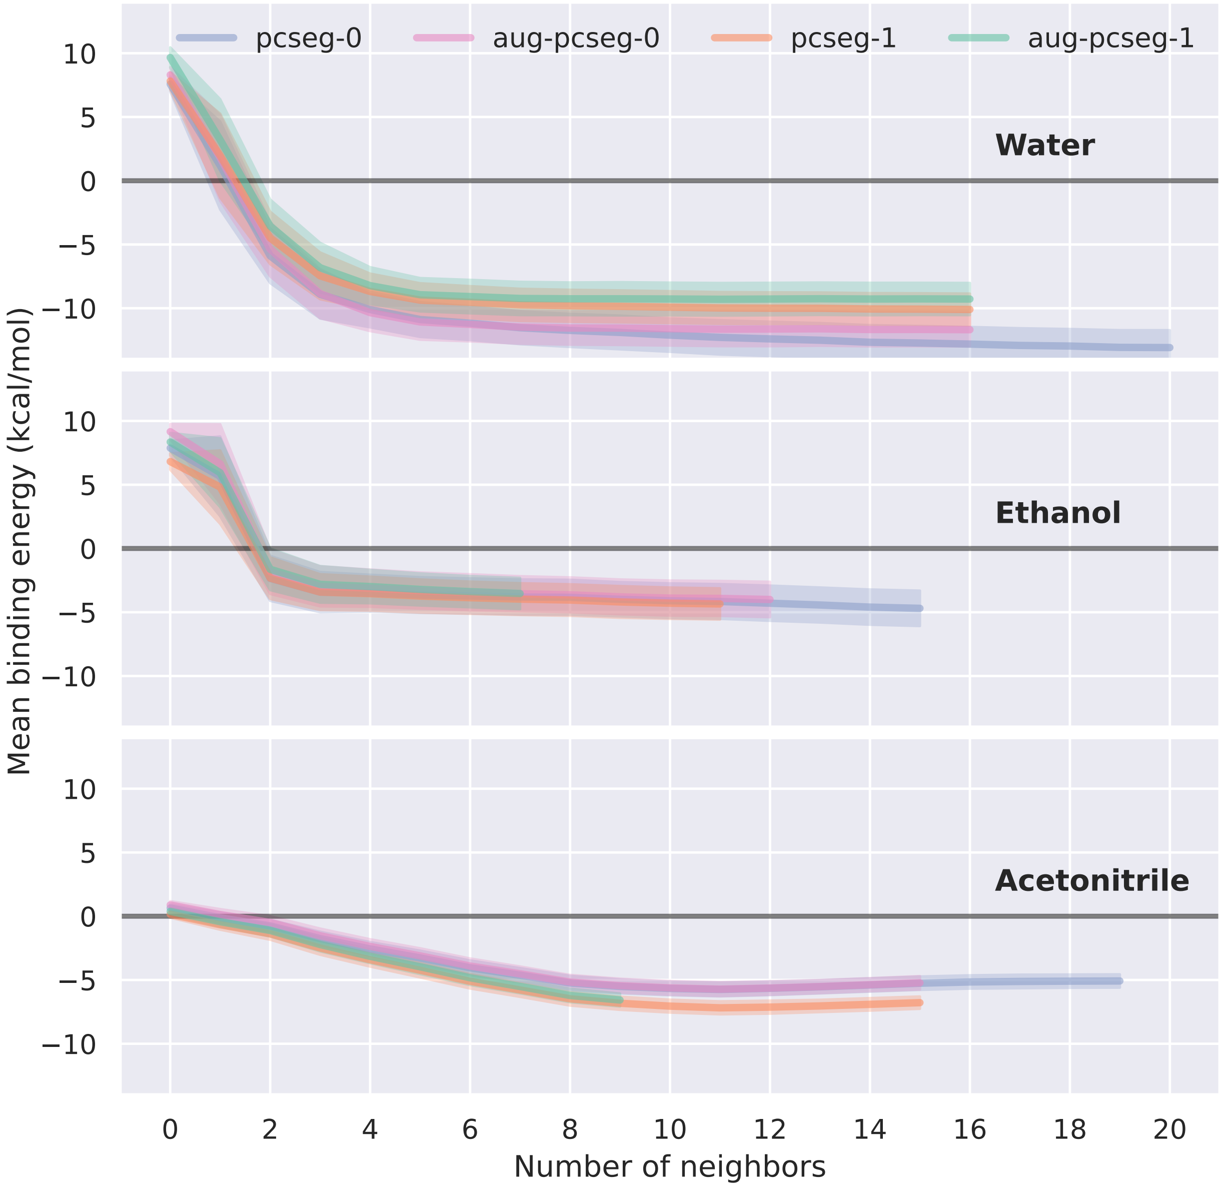


Figure S3: Comparison of different basis sets ($\omega$B97M-V).

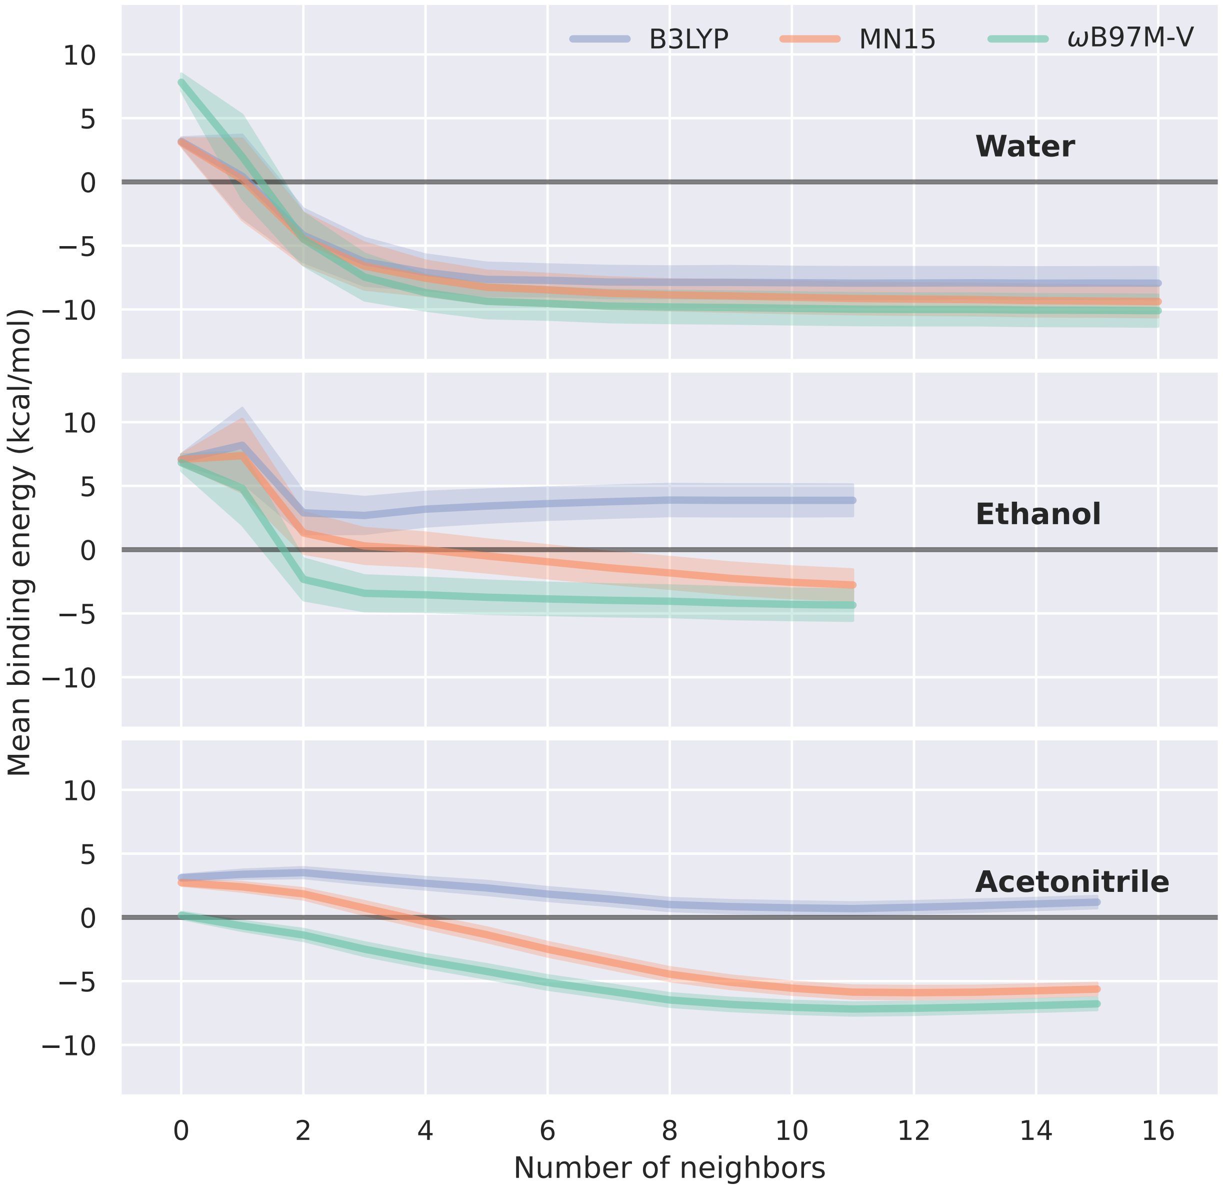


Figure S4: Comparison of different *xc* functionals (pcseg-1).

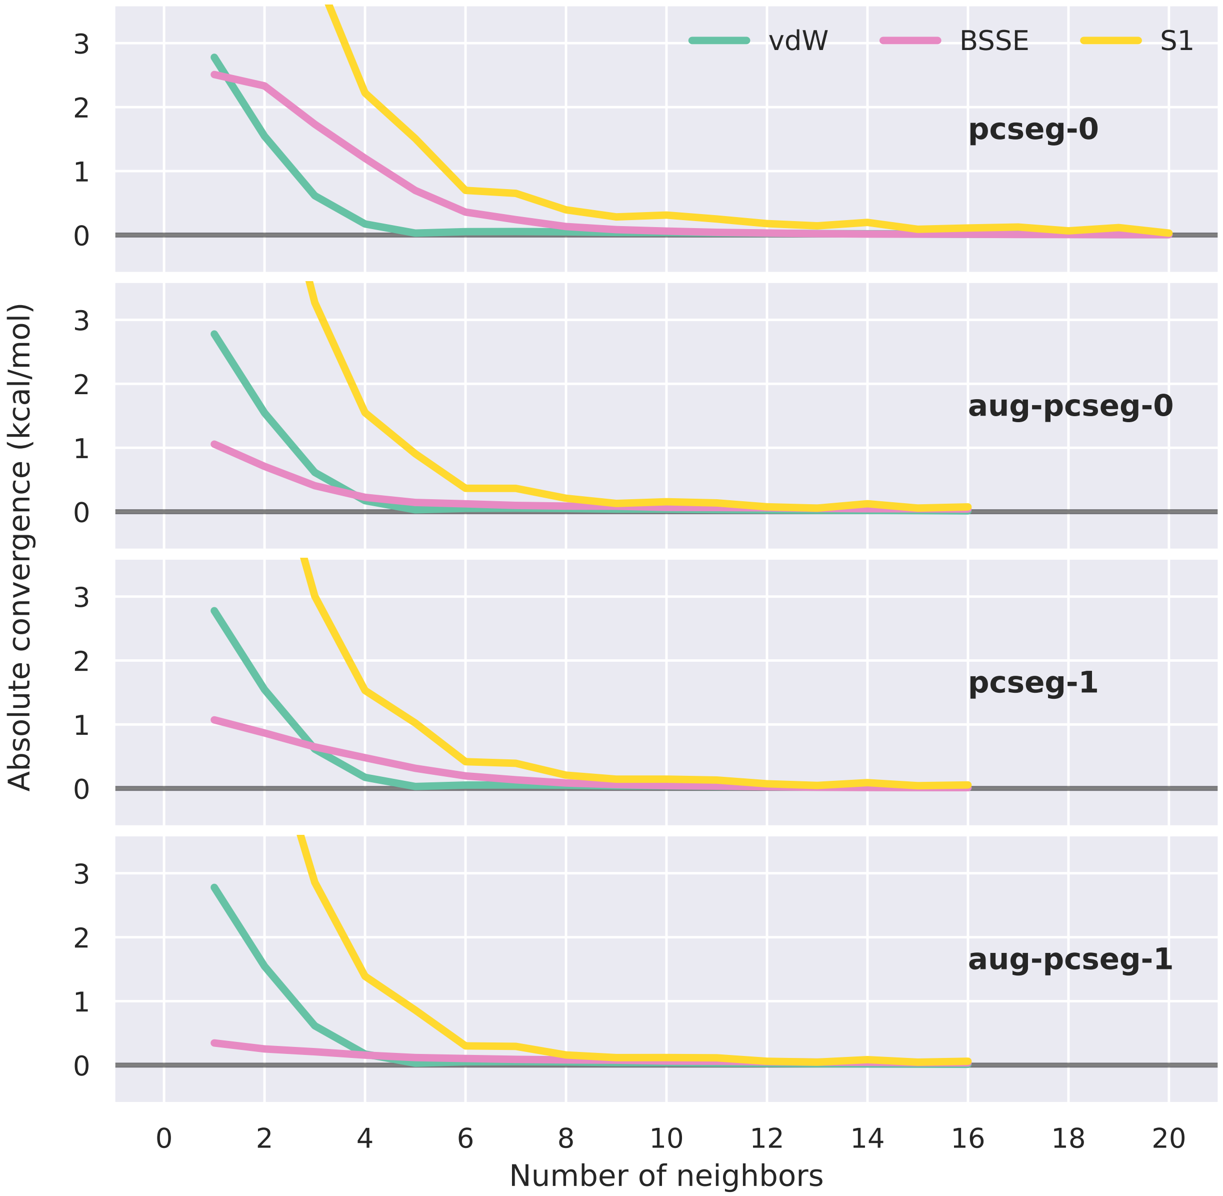


Figure S5: Convergence of individual energy contributions for water ($\omega$B97M-V). The S1, vdW, and BSSE contributions are given in Eqs. S1, S4, and S6, respectively.

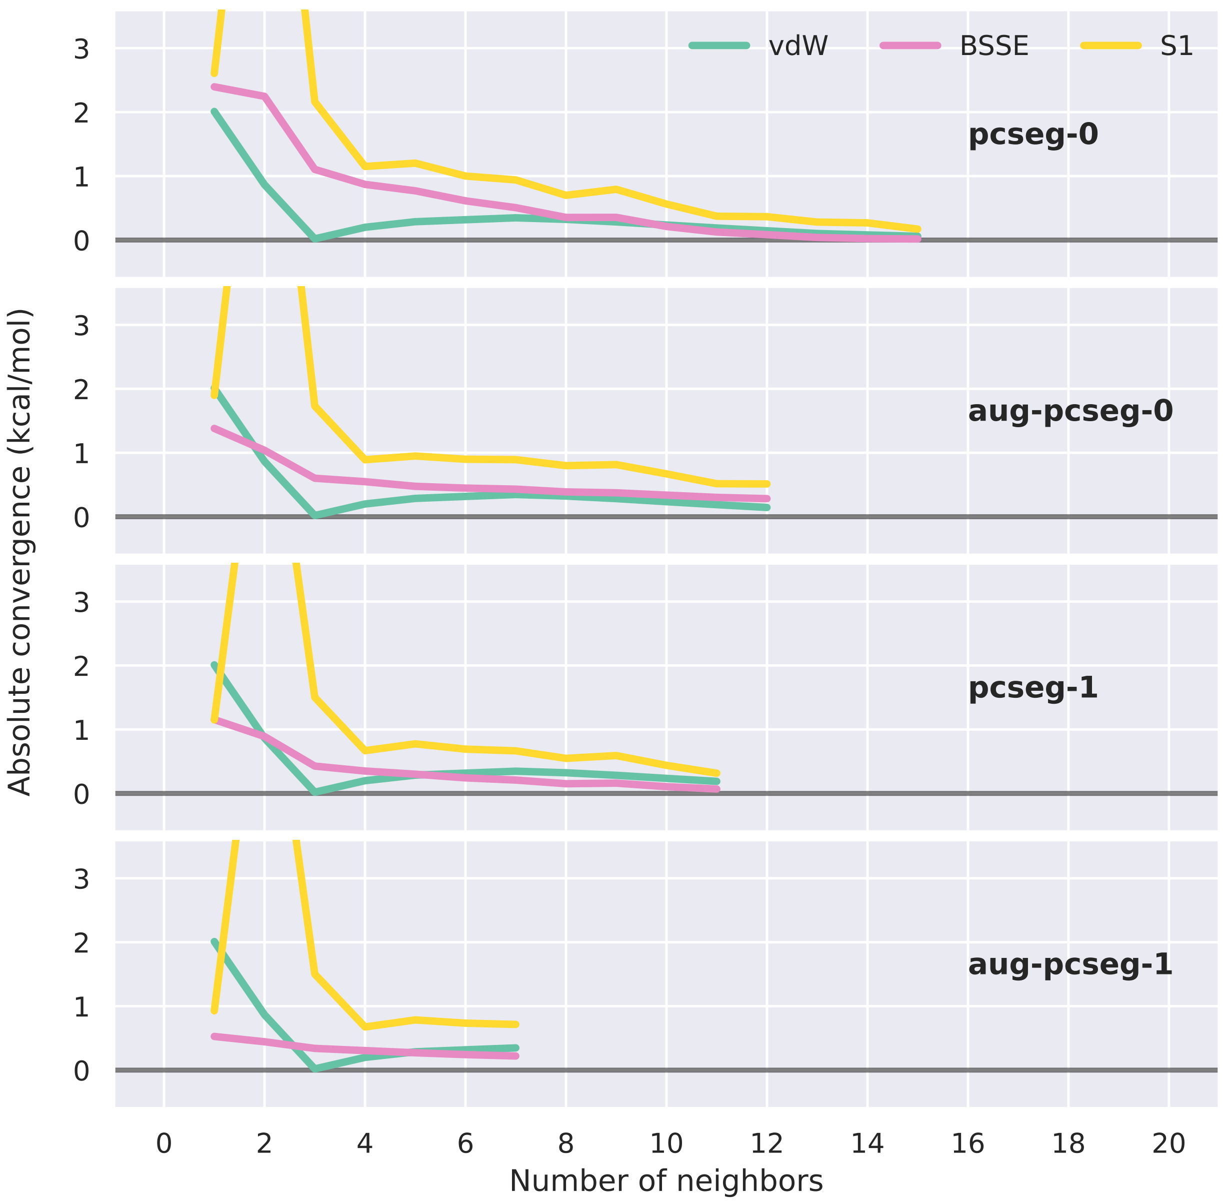


Figure S6: Convergence of individual energy contributions for ethanol ($\omega$B97M-V). Please see the caption to Fig. S5 for further details.

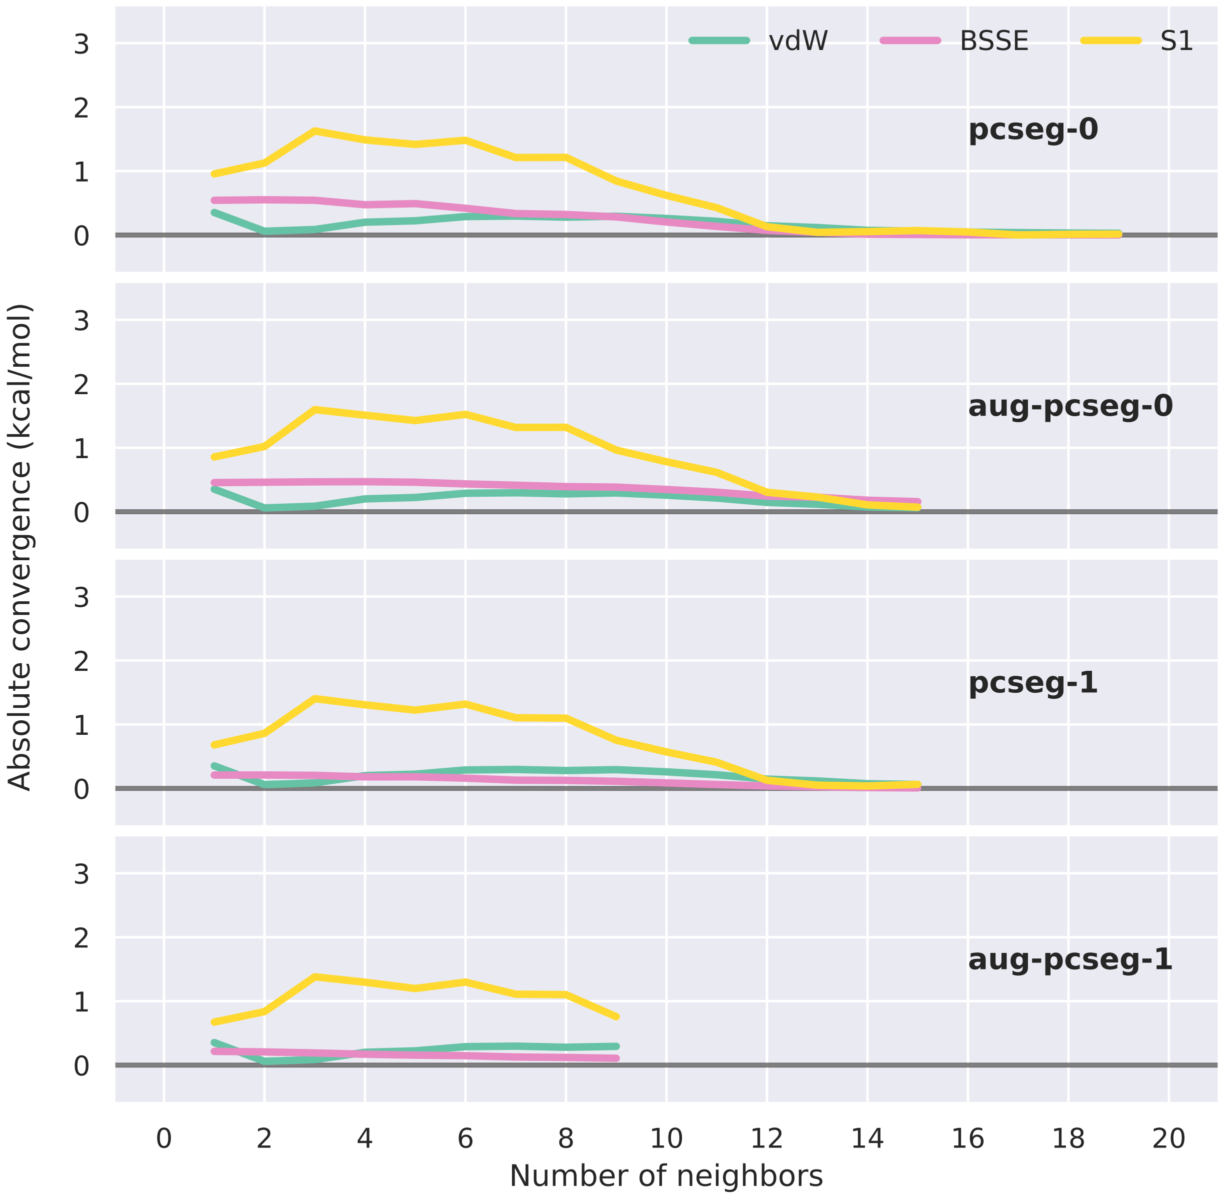


Figure S7: Convergence of individual energy contributions for acetonitrile ($\omega$B97M-V). Please see the caption to Fig. S5 for further details.

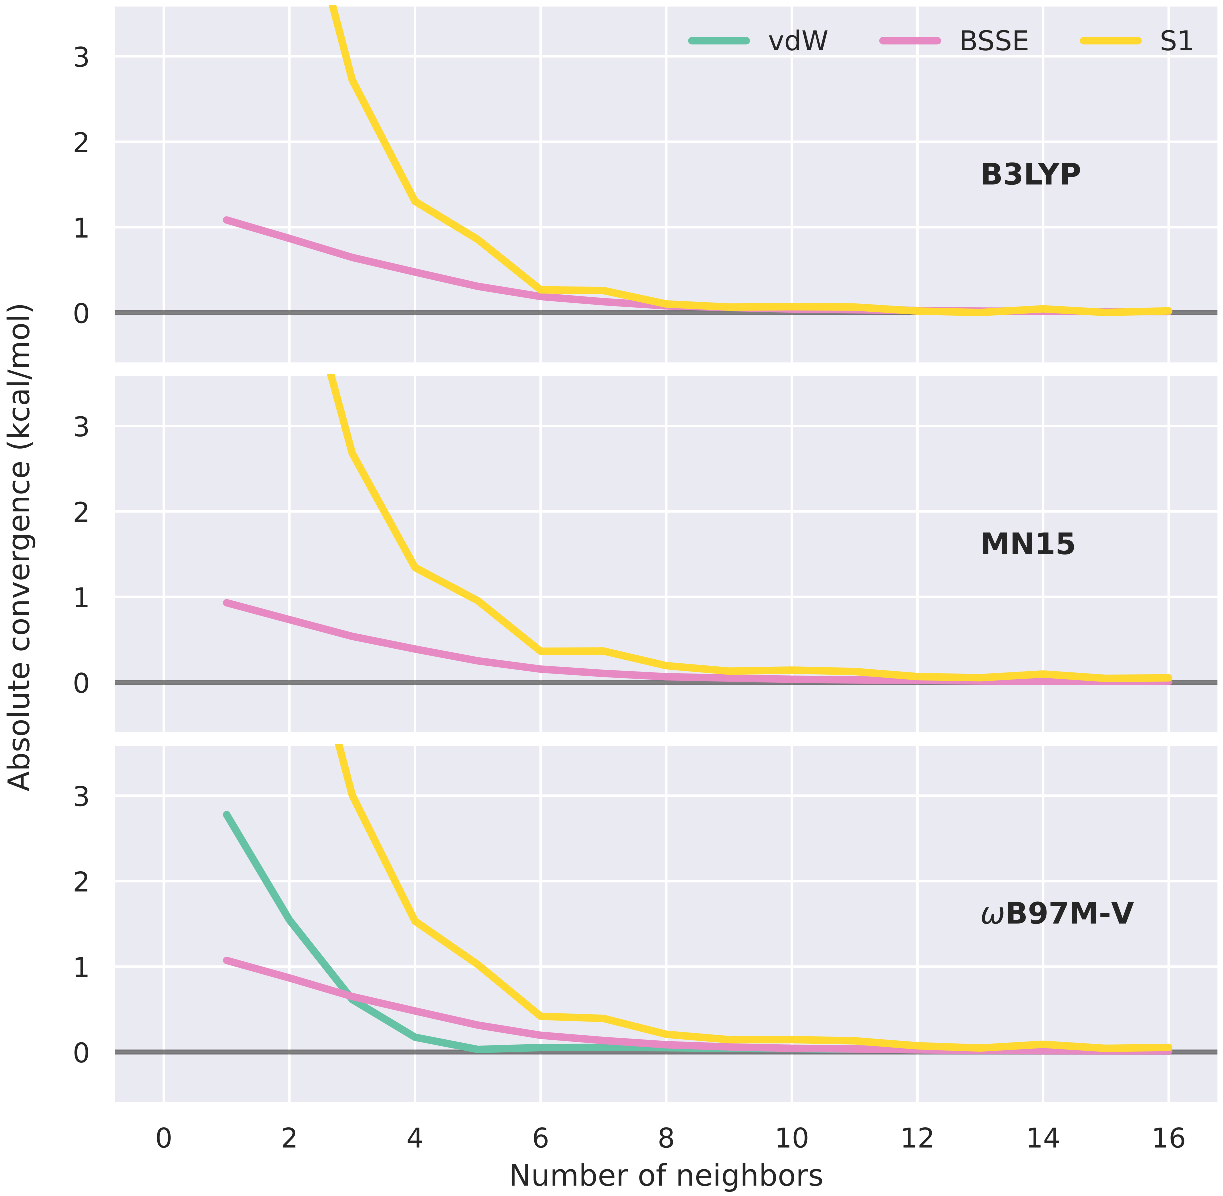


Figure S8: Convergence of individual energy contributions for water (pcseg-1). Please see the caption to Fig. S5 for further details.

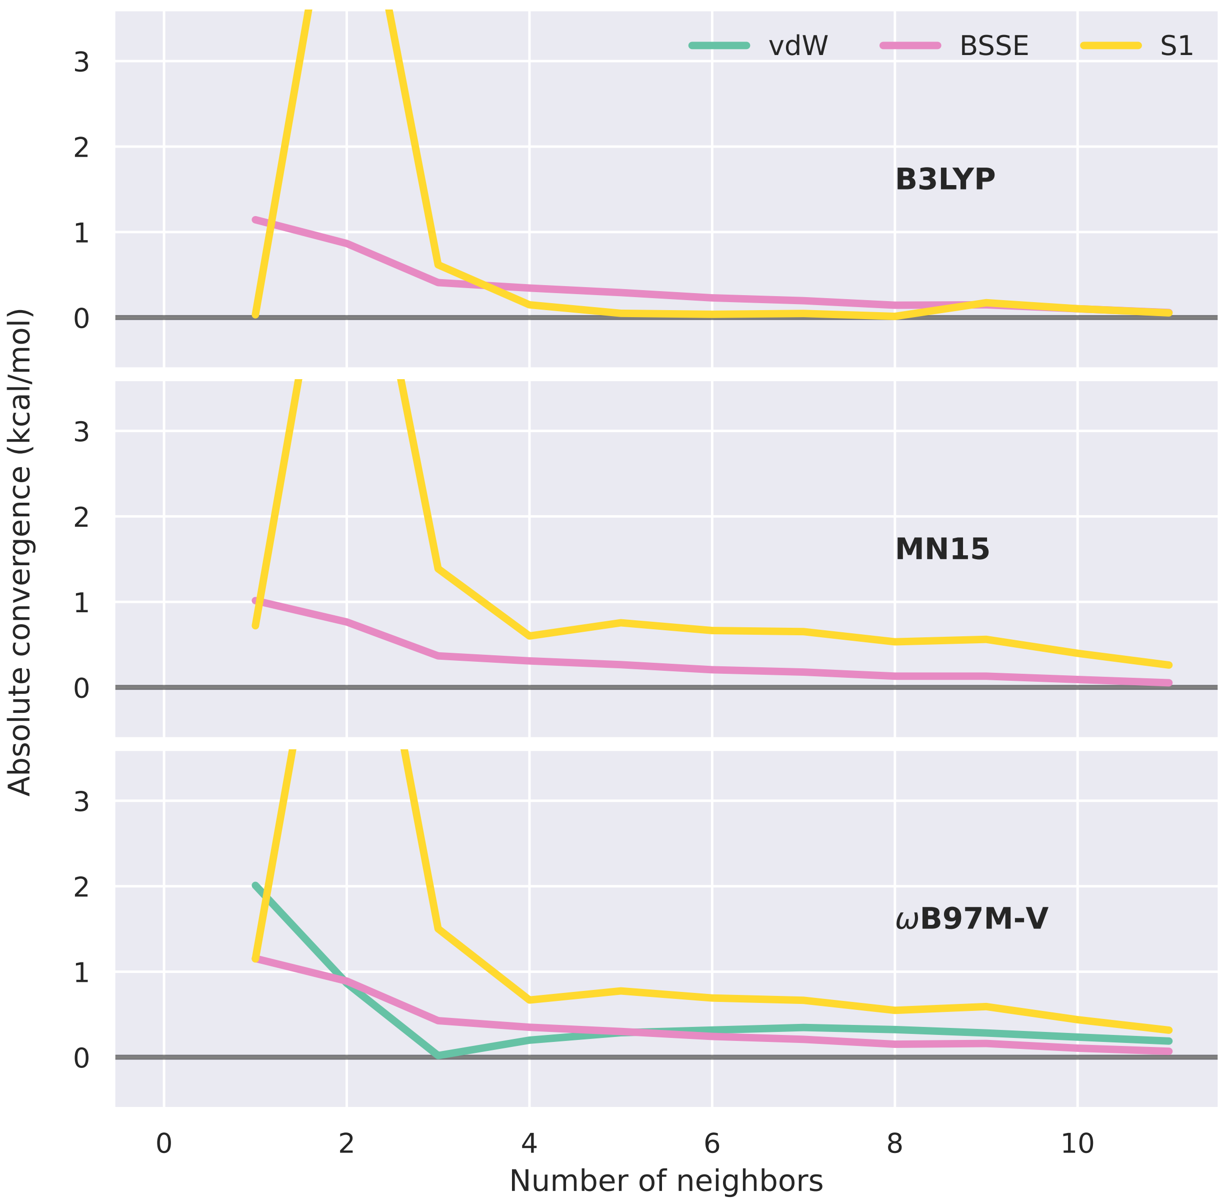


Figure S9: Convergence of individual energy contributions for ethanol (pcseg-1). Please see the caption to Fig. S5 for further details.

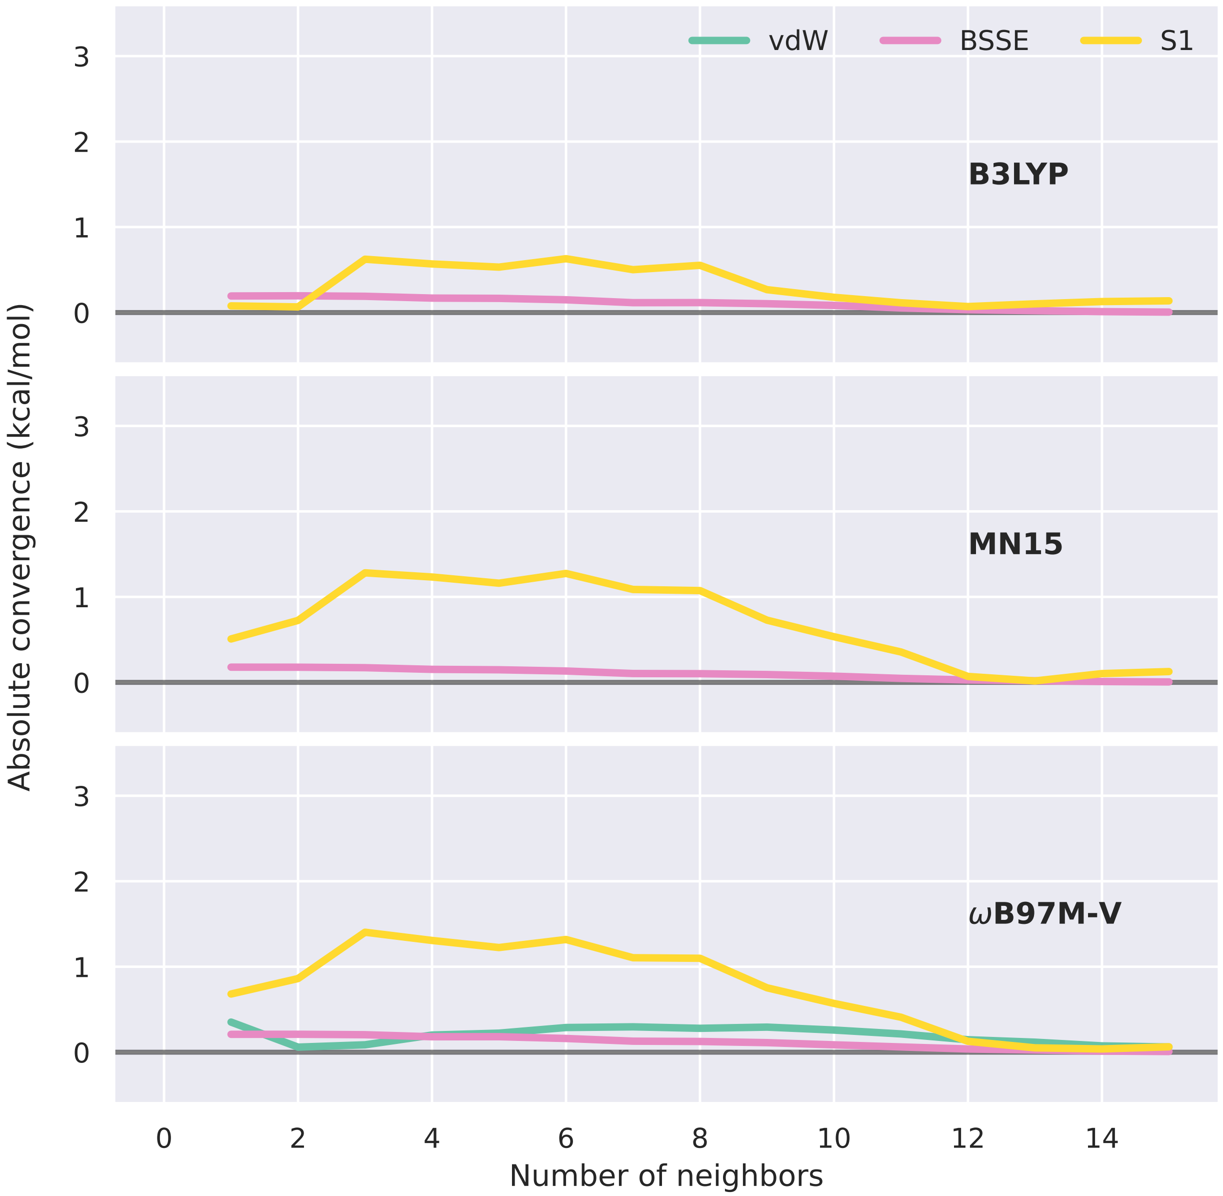


Figure S10: Convergence of individual energy contributions for acetonitrile (pcseg-1). Please see the caption to Fig. S5 for further details.

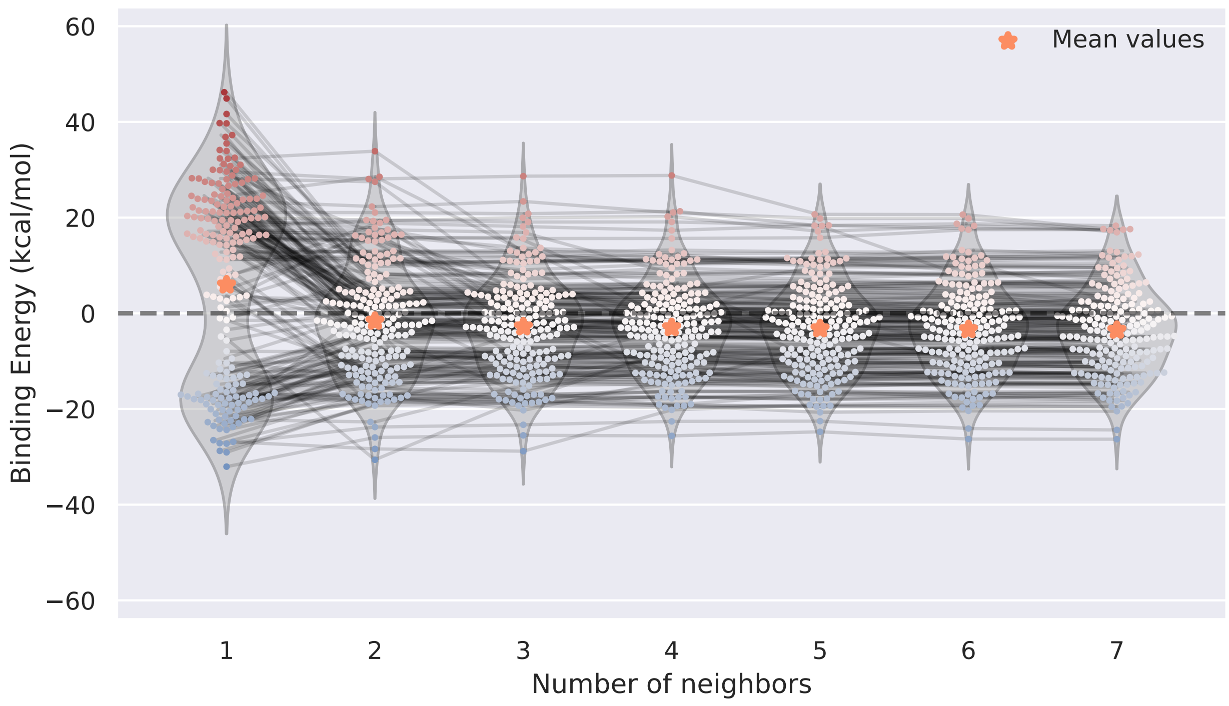


Figure S11: Individual binding energies for ethanol (ωB97M-V/aug-pcseg-1).

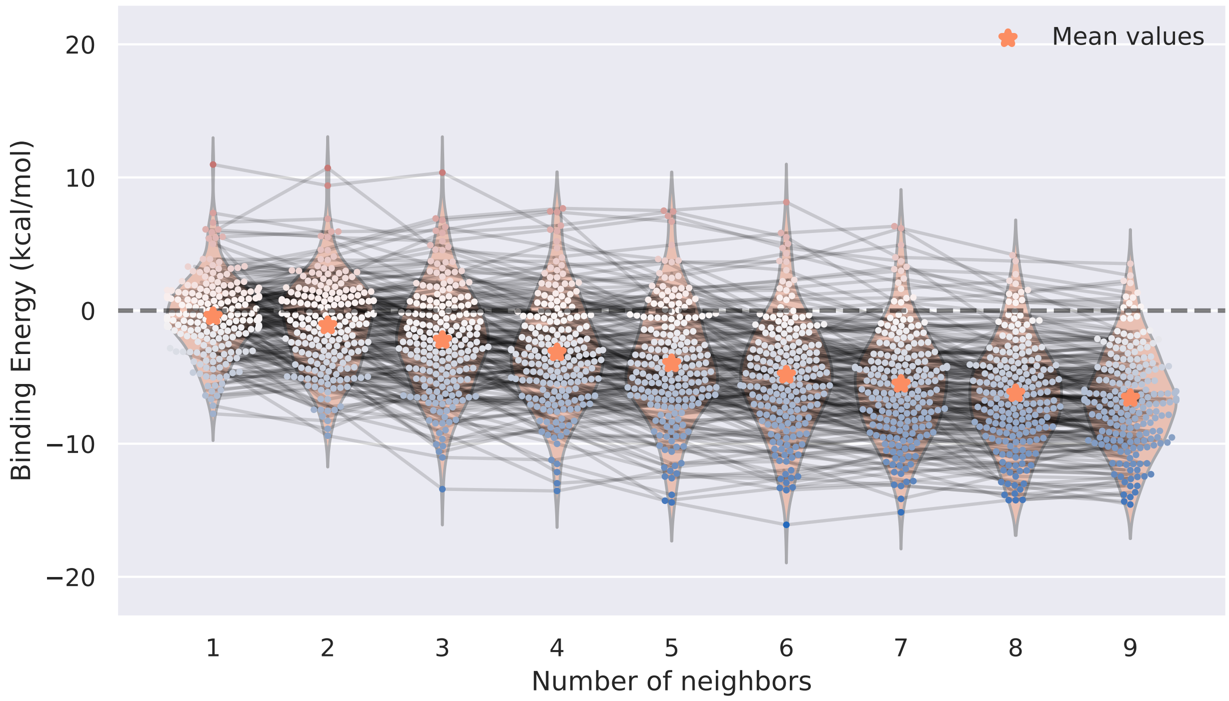


Figure S12: Individual binding energies for acetonitrile (ωB97M-V/aug-pcseg-1).

# References


(S1) Eriksen, J. J. Mean-Field Density Matrix Decompositions. J. Chem. Phys. **2020**, 153, 214109.

(S2) Eriksen, J. J. Decomposed Mean-Field Simulations of Local Properties in Condensed Phases. J. Phys. Chem. Lett **2021**, 12, 6048.

(S3) Eriksen, J. J. Electronic Excitations Through the Prism of Mean-Field Decomposition Techniques. J. Chem. Phys. **2022**, 156, 061101.

(S4) Kjeldal, F. Ø.; Eriksen, J. J. Properties of Local Electronic Structures. J. Chem. Theory Comp. **2023**, 19, 9228.

(S5) Kjeldal, F. Ø.; Eriksen, J. J. Decomposing Chemical Space: Applications to the Machine Learning of Atomic Energies. J. Chem. Theory Comp. **2023**, 19, 2029.

(S6) Kjeldal, F. Ø..; Eriksen, J. J. Transferability of Atom-Based Neural Networks. Mach. Learn.: Sci. Technol. **2024**, 5, 045059.

(S7) Zamok, L.; Eriksen, J. J. Atomic Decompositions of Periodic Electronic-Structure Simulations. J. Phys. Chem. A **2025**, 129, 385.

(S8) Mulliken, R. S. Electronic Population Analysis on LCAO-MO Molecular Wave Functions. I. J. Chem. Phys. **1955**, 23, 1833.

(S9) Mardirossian, N.; Head-Gordon, M. $\omega$B97M-V: A Combinatorially Optimized, Range-Separated Hybrid, Meta-GGA Density Functional with VV10 Nonlocal Correlation. J. Chem. Phys. **2016**, 144, 214110.

(S10) Vydrov, O. A.; Van Voorhis, T. Nonlocal Van Der Waals Density Functional: The Simpler the Better. J. Chem. Phys. **2010**, 133, 244103.

(S11) Ponder, J. W.; Wu, C.; Ren, P.; Pande, V. S.; Chodera, J. D.; Schnieders, M. J.; Haque, I.; Mobley, D. L.; Lambrecht, D. S.; DiStasio, R. A. J.; Head-Gordon, M.; Clark, G. N. I.; Johnson, M. E.; Head-Gordon, T. Current Status of the AMOEBA Polarizable Force Field. J. Phys. Chem. B **2010**, 114, 2549.

(S12) Nakai, H. Energy Density Analysis with Kohn-Sham Orbitals. Chem. Phys. Lett. **2002**, 363, 73.

(S13) Kikuchi, Y.; Imamura, Y.; Nakai, H. One-Body Energy Decomposition Schemes Revisited: Assessment of Mulliken-, Grid-, and Conventional Energy Density Analyses. Int. J. Quant. Chem **2009**, 109, 2464.

(S14) Baba, T.; Takeuchi, M.; Nakai, H. Natural Atomic Orbital Based Energy Density Analysis: Implementation and Applications. Chem. Phys. Lett. **2006**, 424, 193.

(S15) Imamura, Y.; Takahashi, A.; Nakai, H. Grid-Based Energy Density Analysis: Implementation and Assessment. J. Chem. Phys. **2007**, 126, 034103.
